# Supplementary material for: Inverse transition in the two dimensional dipolar frustrated ferromagnet
Source: arXiv:1104.1737 source file (2011-04-09)
Supplement: Supplementary file 1 [file supplementary-material.pdf]

# Supplementary information

## Inverse transition in the two dimensional dipolar frustrated ferromagnet

S. A. Cannas, M. Carubelli, O. V. Billoni and D. A. Stariolo

Here we include the expressions of the variational mean field free energies per unit volume  $f \equiv F/L^2$  used in the work.

### Stripes free energy for $n_{max} = 3$ , used in the calculation of the phase diagram Fig.3

$$\begin{aligned}
 f_s[m_0, \dots, m_3, k_0] = & 2 m_0^2 A(0) + \sum_{n=1}^3 A(nk_0) m_n^2 - 2 h m_0 + \frac{u}{2} [8m_0^4 + 24m_0^2 m_1^2 + 3m_1^4 + 24m_0 m_1^2 m_2 + \\
 & + 24m_0^2 m_2^2 + 12m_1^2 m_2^2 + 3m_2^4 + 4m_1^3 m_3 + 48m_0 m_1 m_2 m_3 + 12m_1 m_2^2 m_3 + 24m_0^2 m_3^2 + \\
 & + 12m_1^2 m_3^2 + 12m_2^2 m_3^2 + 3m_3^4 +]
 \end{aligned} \tag{1}$$

### Bubbles free energy for $n_{max} = 3$ , used in the calculation of the phase diagram Fig.3

$$\begin{aligned}
 f_b[m_0, \dots, m_3, k_0] = & 18 m_0^2 A(0) + 3 \sum_{n=1}^3 A(nk_0) m_n^2 - 6 h m_0 + \frac{u 6^4}{4} \left[ m_0^4 + m_0^2 m_1^2 + \frac{2}{9} m_0 m_1^3 + \frac{5}{72} m_1^4 + \frac{1}{3} m_0 m_1^2 m_2 \right. \\
 & + \frac{1}{9} m_1^3 m_2 + m_0^2 m_2^2 + \frac{2}{9} m_1^2 m_2^2 + \frac{2}{9} m_0 m_2^3 + \frac{5}{72} m_2^4 + 24m_1^3 m_3 + \frac{2}{3} m_0 m_1 m_2 m_3 + \frac{1}{9} m_1^2 m_2 m_3 + \\
 & \left. + \frac{1}{6} m_1 m_2^2 m_3 + m_0^2 m_3^2 + \frac{1}{6} m_1^2 m_3^2 + \frac{1}{9} m_1 m_2 m_3^2 + \frac{1}{6} m_2^2 m_3^2 + \frac{2}{9} m_0 m_3^3 + \frac{5}{72} m_3^4 \right]
 \end{aligned} \tag{2}$$

### Stripes and bubbles free energies for $n_{max} = 1$

$$f_s[m_0, m_1] = 2 m_0^2 A(0) + A(k_m) m_1^2 - 2 h m_0 + \frac{u}{2} [8m_0^4 + 24m_0^2 m_1^2 + 3m_1^4] \tag{3}$$

$$f_b[m_0, m_1] = 18 m_0^2 A(0) + 3A(k_m) m_1^2 - 6 h m_0 + \frac{u 6^4}{4} \left[ m_0^4 + m_0^2 m_1^2 + \frac{2}{9} m_0 m_1^3 + \frac{5}{72} m_1^4 \right] \tag{4}$$

The one mode phase diagram from the inset of Fig.3 (compare with Fig.2 of Ref.[7] and Fig.4 of Ref.[13]) is obtained from these equations (references from the manuscript). They exactly map into Eqs.(8) and (9) of Ref.[7] with the replacement:  $m_0 = m_{s0}/2$ ,  $m_1 = m_s/2$  and  $m_0 = m_{B0}/6$ ,  $m_1 = m_B/2$  into Eqs.(3)

and (4) respectively. With an appropriated rescaling of the variables they also map into Eqs.(21) and (22) of Ref.[13].

**Stripes free energy at zero field (only modes with odd  $n$  contribute) for  $n_{max} = 9$**

$$\begin{aligned}
f_s[m_1, \dots, m_9, k_0] = & A(k_0) m_1^2 + \dots + A(9k_0) m_9^2 + \frac{u}{2} [3m_1^4 + 4m_1^3 m_3 + 12m_1^2 m_3^2 + 3m_3^4 + 12m_1^2 m_3 m_5 + \\
& + 12m_1 m_3^2 m_5 + 12m_1^2 m_5^2 + 12m_3^2 m_5^2 + 3m_5^4 + 12m_1 m_3^2 m_7 + 12m_1^2 m_5 m_7 + \\
& + 24m_1 m_3 m_5 m_7 + 12m_3 m_5^2 m_7 + 12m_1^2 m_7^2 + 12m_3^2 m_7^2 + 12m_5^2 m_7^2 + 3m_7^4 + 4m_3^3 m_9 + \\
& + 24m_1 m_3 m_5 m_9 + 12m_1 m_5^2 m_9 + 12m_1^2 m_7 m_9 + 24m_1 m_3 m_7 m_9 + 24m_3 m_5 m_7 m_9 + \\
& + 12m_5 m_7^2 m_9 + 12m_1^2 m_9^2 + 12m_3^2 m_9^2 + 12m_5^2 m_9^2 + 12m_7^2 m_9^2 + 3m_9^4] \quad (5)
\end{aligned}$$
